# Supplementary material for: Why (and When) does Local SGD Generalize Better than SGD?
Source: arXiv:2303.01215 source file (2023-03-09)
Supplement: Supplementary file 1 [file main_theorem.tex]

\subsection{Statement of main theorem}
Let $\{(\vths_{1, t}, \cdots, \vths_{K, t})\mid   s\geq 0, 0\leq t \leq H\}$ be adapted to a filtration $\{\scrFs_t \mid s \geq 0, 0\leq t \leq H\}$  where $\scrFs_H \subseteq \scrFs[s+1]_0$ and $\scrFs_t \subseteq \scrFs_{t+1}$.
\begin{theorem}[Evaluate the expectation and covariance of one step update]\label{thm: one step moment}
If $\vtheta_0$ is initialized such that ..., then 
\begin{align*}
    \E[\hvphs[(n+1)R_1] -\hvphs[n R_1] \mid \scrFs[nR_1]_{\mathrm{good}}]=XXX,\\
    \E[(\hvphs[(n+1)R_1] -\hvphs[n R_1])(\hvphs[(n+1)R_1] -\hvphs[nR_1])^{\top}\mid \scrFsg[nR_1]]=XXX
\end{align*}
where the constant is independent of $\scrFsg[nR_1]$.
\end{theorem}

\begin{comment}
\begin{align*}
\dd \vzeta(t)=\frac{1}{\sqrt{K}}\mSig_{\parallel}^{1/2}(\vzeta)\dd W(t)+\frac{1}{2K}\partial^2 \Phi(\vzeta)[\mSig(\vzeta)]\dd t+\frac{1}{2}\left(1-\frac{1}{K}\right)\partial^2 \Phi(\vzeta)[\Psi(\mSig(\vzeta))]\dd t, 
\end{align*}
where 
\begin{align*}
     \Psi(\mSig_0)_{i, j} = \begin{cases}
   \left(1 -\frac{1-(1-(\lambda_i+\lambda_j)\eta)^{\alpha / \eta}}{
  \alpha(\lambda_i+\lambda_j)}\right)\Sigma_{0, i, j}\approx \psi(\eta H (\lambda_i + \lambda_j)) \Sigma_{0, i, j}, & \lambda_i >0 \mathrm{\  or\ } \lambda_j>0, \\
    0, &\lambda_i= \lambda_j=0.
    \end{cases}
\end{align*}
Let $\psi(x):=\frac{e^{-x}-1+x}{x}$

\kaifeng{maybe this is a better way to write the above formula:}
Let $B$ be the global batch size.
\begin{align*}
\dd \vzeta(t)=\frac{1}{\sqrt{B}}\mSig_{\parallel}^{1/2}(\vzeta)\dd W(t)+\frac{1}{2B}\partial^2 \Phi(\vzeta)\left[\mSig(\vzeta) + (K-1) \mPsi(\vzeta)\right]\dd t.
\end{align*}
Define 
\begin{align*}
     \mPsi(\vtheta) = \sum_{i, j \in [D]} \psi(\eta H(\lambda_i + \lambda_j)) \left\langle\mSig(\vtheta), \vv_i \vv_j^\top \right\rangle \vv_i \vv_j^\top,
\end{align*}
where $\lambda_i, \vv_i$ are the $i$-th eigenvalue and eigenvector of $\nabla^2 \cL(\vtheta)$,
$\psi(x):=\frac{e^{-x}-1+x}{x}$ and $\psi(0) = 0$.

When $\eta H \to +\infty$, $\mPsi(\vtheta) \to \mSig(\vtheta) - \mSig_{\parallel}(\vtheta)$.

\kaifeng{maybe we can define $\mSig_{\diamond}(\vtheta) := \mSig(\vtheta) - \mSig_{\parallel}(\vtheta)$}
\end{comment}
